# Supplementary material for: Design Concerns for Integrated Scripting and Interactive Visualization in Notebook Environments
Source: arXiv:2205.04557 source file (2024-10-16)
Supplement: Supplementary file 1 [file supplemental_toc.tex]

\section{Supplemental Material Overview}
    The supplemental materials for this work include an supplemental document, zip
archive, a video, and a Github repository.

    The supplemental document contains additional figures, both the visualization and design documents, additional detail regarding the visual design,  additional development details and additional analysis supporting that in the main paper. Specifically, it includes:
    \begin{itemize}
        \itemsep=0ex
        \item A description of how we applied Meyer and Dykes' criteria for rigor~\cite{meyer2019criteria},
        \item Description and figures of our early design mockups, 
        \item Additional development details on the visualization itself, including our algorithm (with comparison figures) for handling labeling clutter to improve tree scalability, design decisions for node elision, and how we show elided subtrees to users,
        \item An elaborated task analysis with justifications drawn from our design notes,
        \item and additional findings from and reflections on our two evaluation studies.
    \end{itemize}

    \noindent The zip archive contains the following documents
    \begin{enumerate}
        \itemsep0em
        \item project\_notes.pdf - The file containing personal notes used by the primary author for design and development of this visualization.
        \item visualization\_evaluation - A directory containing the datasets and notebooks used for our intial visualization evaluation along with a PDF file detailing our evaluation design (EvaluationDesign.pdf), a PDF file containing our evaluation script (EvaluationScript.pdf) and the merged-codes resulting from evaluation sessions (merged-codes.pdf).
        \item visualization\_scripting\_study -  A directory containing the datasets and notebooks used for our followup visualization-scripting study along with a PDF file detailing our study design (Evaluation 2 Planning.pdf) and a PDF file containing our study script (Evaluation 2 Script.pdf). Additionally, codes and analysis resulting from the studies from each visualization researcher are contained in the file ``R2-theme-analysis.pdf" and the directory ``R1 - Codes and Notes".
    \end{enumerate}

    \noindent The video contains:
    \begin{itemize}
        \itemsep0em
        \item A brief overview of the problem we are addressing,
        \item A high level introduction to the our visualization/scripting task analysis,
        \item and usage examples of the interactive tree visualization, automatic updating functionality and linked views.
    \end{itemize}
    
    Source code for the software used for this evaluation can be found at: https://github.com/cscully-allison/hatchet-llnl/tree/vis-working
